# Supplementary material for: Curvature-driven AC-assisted creep dynamics of magnetic domain walls
Source: arXiv:2012.09377 ancillary file (2020-12-17)
Supplement: Supplementary file 1 [file SupMatdef.pdf]

# Supplemental Material for: Curvature driven AC assisted creep dynamics of magnetic domain walls

P. Domenechini, F. Paris, M. G. Capeluto, M. Granada, J.-M. George, M. G. Capeluto, G. Pasquini, and A. B. Kolton

(Dated: December 16, 2020)

In this supplement we describe in more detail the experimental setup and protocols, and include additional information and details of the analytical and numerical calculations. In Section I, experimental details about samples, experimental setup and protocols, as well as description of the image analysis technique is provided. In Section II we show the DC velocity-field curves, in Section III we summarize the relevant typical micromagnetic parameters for samples used in this work, and in Section IV we show the raw AC-driven time-dependent domain area an perimeter at different fields. All this information is used to experimentally evaluate the quantity $\Lambda$ (Eq. (22)) that we compare directly with the theoretical prediction (main-text Eq. (6) and Eq.(23)), as shown in main-text Figure 4a. In Section V we present the full derivation of the analytical model for the evolution of AC-driven domain area and perimeter, whereas in Section VI A and VI B we derive and discuss in details the resulting zero and first order predictions. In Section VII we describe the numerical simulation method and, in Sections VII A and VII B, we show numerical results that validate the analytical model. Finally, as an interesting by-product of our phenomenological theory, in Section VIII a discussion about the extraordinary stability of a circular magnetic domain in Pt/Co/Pt thin-film ferromagnets is included.

## CONTENTS

I. Experimental details 1
A. Samples 1
B. Experimental setup 1
C. Image analysis technique 2
D. Experimental Protocols 2

II. Velocity-field curves 3

III. Micromagnetic parameters 3

IV. AC evolution 4

V. Model details 4

VI. Predictions Details 6
A. Order zero 6
B. First Order 6

VII. Numerical Validation of the model 6
A. Spontaneous and ac-assisted collapse dynamics without pinning 7
B. AC-assisted collapse dynamics with pinning 8

VIII. How stable are circular domains? 10
A. Without pinning 10
B. With pinning 10

References 11

## I. EXPERIMENTAL DETAILS

### A. Samples

In this section we include some details regarding the two kinds of samples used in this work: the sample called S1 in the main text is a Pt(8 nm)/Co(1 nm)/Pt(4 nm) film, containing one magnetic Co layer, grown by DC magnetron sputtering on naturally oxidized (001) Si substrates at room temperature, as detailed in Refs. 1 and 2. The sample called S2 is a Pt(6 nm)/[Co(0.2 nm)/Ni(0.6 nm)]$_4$/Al(5 nm) containing a magnetic CoNi multilayer (the number in parenthesis indicates the thickness of each layer), grown on oxidized Si-SiO$_2$ substrates by DC magnetron sputtering as described in Ref. 3.

Both samples display strong perpendicular magnetic anisotropy (PMA) that was evidenced by DC out-of-plane magnetization measurements, using a vibration VMS magnetometer, and by Local magnetization loops, obtained by means of PMOKE microscopy observations. Figure 1 shows local out-of-plane hysteresis loops measured in both samples by applying successive 50 ms magnetic field pulses of increasing (decreasing) amplitudes up to $\pm 250$ Oe.

### B. Experimental setup

Magneto-optical images were obtained at room temperature, with a home-made polar magneto-

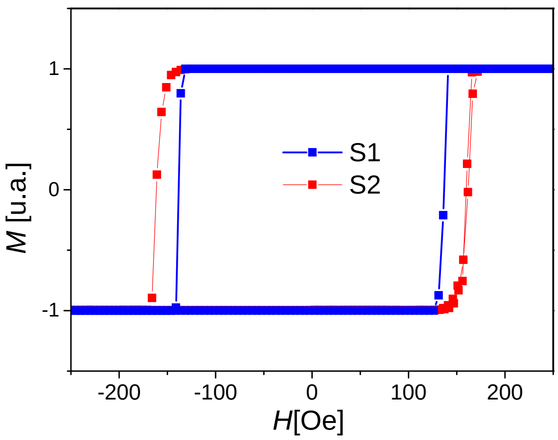


Figure 1. Local magnetic hysteresis loops measured by PMOKE microscopy in both samples, displaying a sharp squared shape, typical of systems with PMA

optical Kerr effect (PMOKE) microscope in the Köhler configuration, using as light source a LED with a central wavelength of 650 nm. Two polarizers were included in the excitation and collection optical paths. 10× amplified images were obtained with a 12 bits CCD camera, with 0.39 $\mu$m/pixel spatial resolution. Specially designed Helmholtz coils allowed us to apply square magnetic field pulses with amplitude $H$ up to 700 Oe and duration $\tau > 1$ ms, in the direction normal to the sample, with an homogeneity of $\Delta H/H < 0.04$ in a 0.126 mm$^2$ area.

### C. Image analysis technique

Due to the relatively low contrast obtained in the raw images, a four-step image processing was performed by applying the following steps sequentially. First, an image of the fully saturated sample was subtracted pixel by pixel from the image of a growth domain (panel (a) in Figure 2). Second, the contrast of the resulting image was increased by applying a non-linear filter, mapping the intensity as $I(x,y) = \tanh(f(x,y)/I_{max})$, where $f(x,y)$ is the intensity of each pixel, and $I_{max}$ is the maximum intensity of the subtracted image (panel (b)). In the third step the noise on the image was reduced by applying a moving average media filter. Finally, in the fourth step, the image was binarized (panel (c)). As it can be clearly seen in panel (c), by the superposition of the domain wall profile taken from the binarized image and the subtracted background image, there is not significant loss of information in the DW during this process.

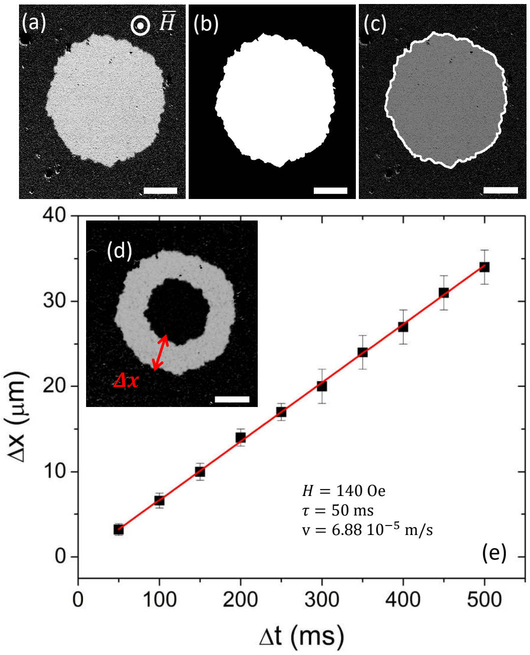


Figure 2. The upper panels show example of image processing: (a) Image of a magnetic domain obtained after background subtraction (saturated sample). (b) After applying a threshold averaging filter a binary image is constructed, that allows to obtain the DW contour. (c) Superposition of the resulting DW profile, indicated as a white line, and the original image (panel a). The lower panels illustrate the procedure followed to determine the DW mean velocity. Panel (d) shows the displacement $\Delta x$ of the DW after $N$ DC pulses of duration $\tau$ each. The velocity is obtained from the linear fit of $\Delta x$ against the total time $\Delta t = N\tau$ (panel (e)). The scale bar in panels a-d is 40 $\mu$m width.

### D. Experimental Protocols

As mentioned in the main text, due to the DW velocity scales involved, DW dynamics was characterized with a quasistatic technique in which the structure of the domains remains stable during image acquisition. Therefore, images of magnetic domains are taken in zero field after applying magnetic field square pulses that expand (or reduce) the domains.

Domains are grown with a standard method, called in this context a "DC protocol": the sample is full saturated by applying a magnetic pulse of relatively long duration (for example a 200 Oe pulse

with 50 ms is enough in the present samples). A second much shorter nucleation pulse is applied (approximately 150 Oe with times between 1 to 5 ms in the present samples) and then the domain is grown by applying successive pulses of variable amplitude and duration. This protocol was used to measure the velocity-field curves, and also to prepare an initial state to study the AC dynamics.

The AC dynamics was examined with the called "AC protocol" described in the main text. All the results presented in this work were obtained starting from a similar initial condition, a DC growth domain with an area around 4600 $\mu m^2$. The AC amplitudes $H = H_\uparrow > 0$ and $H = -H_\downarrow < 0$ and the corresponding half periods $\tau_1$ (see main text) where chosen in order to obtain in all the cases a mean displacement during each half-cycle of $d \sim 6$ $\mu$m. Due the statistical character of the phenomena, each procedure was repeated several times and then averaged (typically ten repetitions are enough to have a reliable mean value).

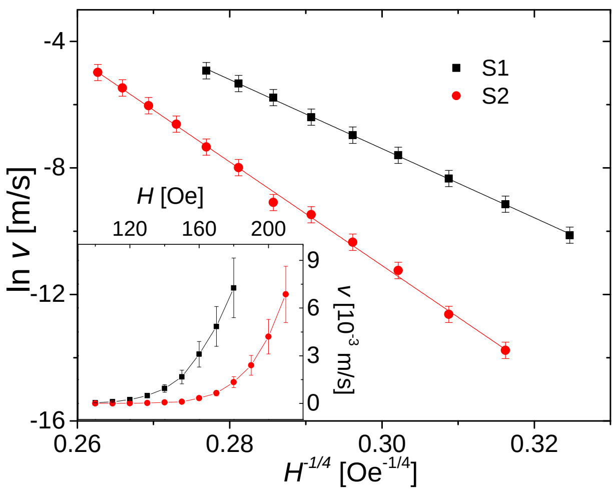


Figure 3. Inset: Dependence of velocity $v$ on applied magnetic field $H$ for samples S1 (black symbols) and S2 (red symbols). Main panel: $\ln v$ against $H^{-1/4}$. The linear behavior indicates that both systems are in the creep regime.

## II. VELOCITY-FIELD CURVES

To obtain the dependence of the mean DW velocity with the applied magnetic field ($v(H)$ curves), the "DC protocol" is applied to an initially domain grown to an area around 1000 $(\mu\text{m})^2$. To measure the mean DW velocity, successive images taken after applying each magnetic field pulse were subtracted from one another and the mean displacement was measured (see panel (d) in Fig. 2). The time interval $\tau$ was chosen in such a way that the domains grew in small steps without reaching the magnetic saturation of the sample. In Fig. 2(e) the displacement after $N$ DC pulses is plotted against the total time duration $\Delta t = N\tau$. The velocity is then determined from the slope of a linear fit of the displacement data plotted against the total time.

Field amplitudes ranging between 90 and 200 Oe, with period $\tau$ between 500 to 5 ms were applied in both samples. The velocities for each sample shown in the inset of figure Figure3, are an average on ten experimental realizations for each magnetic field. In the main panel the same data are plotted as $ln(v)$ as a function of $H^{-\frac{1}{4}}$, displaying the universal linear behavior expected in the creep regime.

## III. MICROMAGNETIC PARAMETERS

Typical energy and length scales, computed from micromagnetic parameters from both kinds of samples are presented in Table I. The anisotropy constant $K$, saturation magnetization $M_S$ and exchange constant $A$ were extracted from Refs.[4] and [3] for Pt/Co/Pt and Pt/[CoNi]/Pt multilayers, respectively. The surface tension $\sigma$ and Young-Laplace consant $C$ were estimated from given micromagnetic parameters.

| Parameter | Formula | Units | Pt/Co/Pt | CoNi multilayer |
|---|---|---|---|---|
| Anisotropy constant | $K$ | kJ/m$^3$ | 364 | 340 |
| Saturation magnetization | $M_S$ | kA/m | 910 | 540 |
| Exchange constant | $A$ | pJ/m | 14 | 15 |
| DW energy density | $\sigma = \sqrt{AK}$ | mJ/m$^2$ | 2.26 | 2.26 |
| Young Laplace constant | $C = \sigma/2M_S$ | Oe cm | 1.2 $10^{-3}$ | 2.1 $10^{-3}$ |

Table I. Typical micromagnetic parameters for Pt/Co/Pt and Pt[CoNi]−4Pt, representative of samples S1 and S2 respectively.

## IV. AC EVOLUTION

As mentioned in Section I D, due the statistical character of the AC evolution, each procedure was repeated several times. The mean values of the area $A(N)$ and the perimeter $P(N)$, were determined by computing the average of the area and perimeter measured after applying $N$ pulses. The statistical variance of each set of data is assumed as an estimation of the uncertainty in the measurement. Figure 4(a)-(b) shows results obtained for the evolution of the area $A(N)$ and perimeter $P(N)$ used to compute the variable $\Lambda(N)$, plotted in the main-text Figure 4a. It can be seen that, in spite of the decrease in $A(N)$, $P(N)$ slightly grows with $N$, due to the domain deformation.

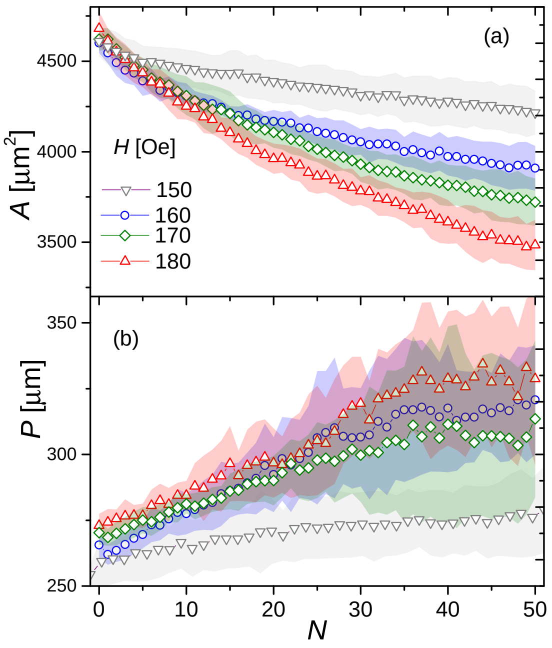


Figure 4. (a) Area and (b) Perimeter evolution as a function of the number of applied AC pulses, measured in sample S2 for different magnetic field amplitudes.

## V. MODEL DETAILS

The area $A_t$ and perimeter $P_t$ time evolution of a plane simple time-dependent closed-curve $\Gamma_t$ (or Jordan curve) is exactly described by

$$\frac{dA_t}{dt} = \int_{\Gamma_t} v_t(\mathbf{r}_s) ds \tag{1}$$

$$\frac{dP_t}{dt} = -\int_{\Gamma_t} v_t(\mathbf{r}_s)\kappa_t(\mathbf{r}_s) ds \tag{2}$$

with $ds$ is the differential arc length along $\Gamma_t$, $v_t(\mathbf{r})$ the local normal velocity and $\kappa_t(\mathbf{r})$ the signed local curvature at the point $\mathbf{r}$ in $\Gamma_t$ at time $t$,

To model a domain wall (DW) in a disordered ferromagnet with the general Eqs. (1) and (2) we will assume they behave as a thin elastic curve $\Gamma_t$ whose normal velocity arises from a local instantaneous response function $v_t \approx R_T(H_t + C\kappa_t(\mathbf{r}), \mathbf{r})$, where $R_T(h_t, \mathbf{r})$ is the local coarse-grained velocity response under the action of a uniform time-dependent field $h_t$ at temperature $T$. In our case $h_t = H_t + C\kappa_t(\mathbf{r})$. The explicit $\mathbf{r}$ dependence in $R_T$ models the disorder-induced local response heterogeneity that survives spatial coarse graining, while thermal noise is completely averaged-out and absorved in the $T$ dependence of $R_T$. This approach is also local in time, so we are assuming that, at the considered time and length coarse-graining scales, transients in the normal velocity at $\mathbf{r}$ can be neglected. In other words, the aproximation is to assume that $v_t$ instantaneously responds to the instanraneous local curvature and to the external field. Note however that the whole curve can evolve in a non-steady manner which may depend not only on the external fields and quenched disorder but on its initial condition as well.

Under the above assumptions the equations for $P_t$ and $A_t$ read

$$\frac{dA_t}{dt} = \int_{\Gamma_t} R_T(H_t + C\kappa_t(\mathbf{r}_s), \mathbf{r}_s) ds \tag{3}$$

$$\frac{dP_t}{dt} = -\int_{\Gamma_t} R_T(H_t + C\kappa_t(\mathbf{r}_s), \mathbf{r}_s)\kappa_t(\mathbf{r}_s) ds. \tag{4}$$

These equations are unfortunately non-closed as they require the knowledge of the local instantaneous signed curvature at each point $\mathbf{r}_s$ in $\Gamma_t$. We can nevertheless make progress doing two extra approximations. We first neglect heterogeneity at the coarse-grained level and assume that $R_T(H_t + C\kappa_t(\mathbf{r}), \mathbf{r}) \approx V_T(H_t + C\kappa_t(\mathbf{r}))$, with $V_T(h)$ the DW velocity-field characteristics. We thus obtain

$$\frac{dA_t}{dt} \approx \int_{\Gamma_t} V_T(H_t + C\kappa_t(\mathbf{r}_s)) ds \tag{5}$$

$$\frac{dP_t}{dt} \approx -\int_{\Gamma_t} V_T(H_t + C\kappa_t(\mathbf{r}_s))\kappa_t(\mathbf{r}_s) ds. \tag{6}$$

Note that within this homogeneous approximation we are not neglecting disorder, as it is partially absorbed in $V_T$, which has a very different behaviour in presence of disorder. In particular, it becomes temperature dependent and strongly non-linear. Second, we will assume that $H_t \gg C\kappa_t(\mathbf{r})$, an assumption that can be well fulfilled experimentally. Indeed, typical domains are found to be ultra-stable if $H_t = 0$ (i.e. only driven by curvature pressure), while applied fields amplitudes $H_t$ are usually tuned such that the motion is observable by PMOKE microscopy.

From the above assumptions, by writing

$$V_T(H_t + C\kappa) \approx V_T(H_t) + V_T'(H_t)C\kappa_t(\mathbf{r}_s) + \frac{V_T''(H_t)}{2}C^2\kappa_t^2(\mathbf{r}_s) + ... \tag{7}$$

with $V_T'$ and $V_T''$ the derivatives with respect to field of $V_T$, we can now develop perturbatively the differential equations for $A_t$ and $P_t$,

$$\frac{dA_t}{dt} \approx \frac{dA_t^{(0)}}{dt} + \frac{dA_t^{(1)}}{dt} + \frac{dA_t^{(2)}}{dt} + ..., \tag{8}$$

where

$$\begin{aligned} \frac{dA_t^{(0)}}{dt} &= V_T(H_t)P_t, \\ \frac{dA_t^{(1)}}{dt} &= -2\pi C V_T'(H_t), \\ \frac{dA_t^{(2)}}{dt} &= \frac{C^2 V_T''(H_t)}{2} P_t \langle \kappa_t^2 \rangle. \end{aligned} \tag{9}$$

To get these expressions we used that $P_t = \int_{\Gamma_t} ds$, the $\Gamma_t$ topological index $\int_{\Gamma_t} \kappa ds = -2\pi$, and defined the mean squared curvature $\langle \kappa_t^2 \rangle \equiv P_t^{-1} \int_{\Gamma_t} \kappa_t^2 ds$ of $\Gamma_t$. We can proceed similarly for $P_t$,

$$\frac{dP_t}{dt} \approx \frac{dP^{(0)}}{dt} + \frac{dP^{(1)}}{dt} + \frac{dP^{(2)}}{dt} + ... \tag{10}$$

where

$$\begin{aligned} \frac{dP_t^{(0)}}{dt} &= 2\pi V_T(H_t), \\ \frac{dP_t^{(1)}}{dt} &= -C V_T'(H_t) P_t \langle \kappa_t^2 \rangle, \\ \frac{dP_t^{(2)}}{dt} &= -\frac{C^2 V_T''(H_t)}{2} P_t \langle \kappa_t^3 \rangle. \end{aligned} \tag{11}$$

As described in Section I D, the applied AC-field in the experiments consists in alternated square pulses of identical duration $\tau_1$ and amplitude $H = H_\uparrow > 0$ and $H = -H_\downarrow < 0$, respectively. The two pulses are periodically repeated with period $\tau \geq 2\tau_1$.

To derive useful formulas to deal with the AC response let us consider a function $X_t$ with a very smooth variation in any single period $\tau$ and a given function $f(x)$ and calculate the following integral in one period of the AC field:

$$I_n \equiv \int_{n\tau}^{(n+1)\tau} f(H_t)X_t. \tag{12}$$

Using the trapezoidal rule we have

$$\begin{aligned} I_n \approx \{&f(H_\uparrow)[X_{n+1/2} + X_n] \\ &+ f(-H_\downarrow)[X_{n+1/2} + X_{n+1}]\}\frac{\tau}{4} \end{aligned} \tag{13}$$

If we now assume a small pulse assymetry $\Delta H = H_\uparrow - H_\downarrow$, such that $f(-H_\downarrow) \approx f(-H_\uparrow) + f'(-H_\uparrow)\Delta H$, we can write

$$\begin{aligned} I_n \approx\ &f(H_\uparrow)[X_n + X_{n+1/2}]\frac{\tau}{4} \\ &+ f(-H_\uparrow)[X_{n+1/2} + X_{n+1}]\frac{\tau}{4} \\ &+ f'(-H_\uparrow)[X_{n+1/2} + X_{n+1}]\Delta H\frac{\tau}{4}. \end{aligned} \tag{14}$$

We are interested in the cases where $f(x)$ is either odd ($f(x) = -f(-x)$ and $f'(x) = f'(-x)$), or even ($f(x) = f(-x)$ and $f'(x) = -f'(-x)$). In these cases we get

$$I_n = \begin{cases} -f(H)\frac{d\mathcal{X}}{dN}\frac{\tau}{4} + \Delta H f'(H)\mathcal{X}\frac{\tau}{2} & f \text{ odd} \\ f(H)\mathcal{X}\tau - \Delta H f'(H)\mathcal{X}\frac{\tau}{2} & f \text{ even} \end{cases} \tag{15}$$

where $H = H_\uparrow > 0$. and we have defined $\mathcal{X}$ as $d\mathcal{X}/dN = X_{n+1} - X_n$ or $\mathcal{X} = \int_{n\tau}^{(n+1)\tau} dt'\ dX_t/dt$.

Since we are only interested in the smooth evolution of $A_t$ and $P_t$ as a function of the number $N$ of AC-cycles we can apply the rule of Eq. (15) to Eqs. (9) and (11) exploiting the symmetry $V_T(H) = -V_T(-H)$. Doing so we obtain for the area

$$\begin{aligned} \frac{d\mathcal{A}}{dN} &= \frac{d\mathcal{A}^{(0)}}{dN} + \frac{d\mathcal{A}^{(1)}}{dN} + \frac{d\mathcal{A}^{(2)}}{dN}, \\ \frac{d\mathcal{A}^{(0)}}{dN} &= -V_T(H_t)\frac{d\mathcal{P}}{dN}\frac{\tau}{4} + \Delta H\frac{\tau}{2}V_T'(H)\mathcal{P}, \\ \frac{d\mathcal{A}^{(1)}}{dN} &= -2\pi C V_T'(H_t)\tau + \Delta H V_T''(H)\pi C\tau, \\ \frac{d\mathcal{A}^{(2)}}{dN} &= -\frac{C^2\tau}{8}V_T''(H_t)\frac{d}{dN}[\mathcal{P}\langle\kappa_t^2\rangle] \\ &\quad + \Delta H V_T'''(H) C^2 \mathcal{P}\langle\kappa_t^2\rangle\frac{\tau}{4}, \end{aligned} \tag{16}$$

and similarly for the perimeter

$$\frac{d\mathcal{P}}{dN} = \frac{d\mathcal{P}^{(0)}}{dN} + \frac{d\mathcal{P}^{(1)}}{dN} + \frac{d\mathcal{P}^{(2)}}{dN},$$
$$\frac{d\mathcal{P}^{(0)}}{dN} = \pi\tau V_T'(H)\Delta H,$$
$$\frac{d\mathcal{P}^{(1)}}{dN} = \left[-V_T'(H) + V_T''(H)\frac{\Delta H}{2}\right] C\tau\mathcal{P}\langle\kappa^2\rangle,$$
$$\frac{d\mathcal{P}^{(2)}}{dN} = \frac{C^2 V_T''(H)\tau}{8}\frac{d}{dN}[\mathcal{P}\langle\kappa_t^3\rangle] - \Delta H\frac{C^2 V_T'''(H)}{4}\mathcal{P}\langle\kappa_t^3\rangle\tau, \quad (17)$$

## VI. PREDICTIONS DETAILS

### A. Order zero

Equations 16 and 17 are not closed because they need $\langle\kappa_N^2\rangle$ and $\langle\kappa_N^3\rangle$. The exception is the *order zero*,

$$\frac{d\mathcal{A}}{dN} \approx -V_T(H)\frac{d\mathcal{P}}{dN}\frac{\tau}{4} + \Delta H\frac{\tau}{2}V_T'(H)\mathcal{P} \quad (18)$$
$$\frac{d\mathcal{P}}{dN} = \pi\tau V_T'(H)\Delta H \quad (19)$$

For symmetric pulses $\Delta H = 0$ we get $d\mathcal{A}^{(0)}/dN = 0$ and $d\mathcal{P}^{(0)}/dN = 0$ for any AC amplitude $H$. Order zero hence fails to explain the experimental results which show an average drift of $\mathcal{A}$ and $\mathcal{P}$ or "rectification effect" under an AC drive with no bias.

### B. First Order

At *first order* we can get more physical information. On one hand we note that we can still have a stroboscopic stability, $d\mathcal{A}/dN = 0$ , $d\mathcal{P}/dN = 0$ but only with asymmetric pulses with finite $\Delta H = \Delta H^*$, playing the role of a compensating difference for the curvature driven collapse. Solving we get

$$\Delta H^* \approx \frac{2C}{\mathcal{P}/2\pi + V_T''C/V_T'} \approx \frac{2C}{\mathcal{P}/2\pi} \approx \frac{2C}{\mathcal{R}} \quad (20)$$

where in the second equality we used that $V_T'/V_T'' \gg C/\mathcal{P}$ and in the last one used that $2\pi\mathcal{R} \approx \mathcal{P}$ because of the quasi-circular shape of the initial domains. This result points to DW curvature as the responsible for the compensation effect by asymmetric pulses observed experimentally. The elastic Young-Laplace magnetic pressure $-2C/\mathcal{R}$ compensates the difference $\Delta H$ which favours the growth of the domain. Eq.(20) can be explained in a more intuitive way for a circular domains. In such a case $\kappa_t = -1/R_t$ and we have $dR_t/dt \approx V_T(H + \Delta H/2 - C/R_t)$ in the first half period, and $dR_t/dt \approx -V_T(H - \Delta H/2 + C/R_t)$ in the second half. Therefore, if we want to compensate the forward and backward motions we need $\Delta H = 2C/R_t$, if we assume that $R_t$ varies very little during one period. Eq. (20) is the first prediction we test experimentally.

We can now attempt to explain the shrinking of the domain area $\mathcal{A}$ with *symmetric* pulses. Puting $\Delta H = 0$ we get,

$$\frac{d\mathcal{A}}{dN} = -V_T(H)\frac{d\mathcal{P}}{dN}\frac{\tau}{4} - 2\pi C V_T'(H)\tau. \quad (21)$$

We can define

$$\Lambda = -\frac{\mathcal{A} + \mathcal{P}V_T(H)\tau/4}{2\pi V_T'(H)\tau} \quad (22)$$

such that $\Lambda$ gives us direct access to the micromagnetic parameter $C$,

$$\frac{d\Lambda}{dN} = C. \quad (23)$$

This is the prediction we test experimentally in the case of symmetric AC pulses. Note that one simple test-case for applying Eq. (21) is the $H_t = 0$ spontaneous collapse in the free-flow linear response $V_T(H) \approx mH$, with $m$ a mobility constant, at $H_t = 0$. Then, using $N\tau = t$, $\frac{d\mathcal{A}}{dt} = -2\pi Cm$, a result that can be also obtained directly from the topological invariant $\int_{\Gamma_t} ds\ v_t = \int_{\Gamma_t} ds\ mC\kappa_t = -2\pi mC$, which says that any area spontaneously collapses at a uniform rate, independently of the initial condition.

Finally, it is also worth noting that at first-order the dynamics of the perimeter $\mathcal{P}$ for symmetric pulses $\Delta H = 0$ reads

$$\frac{d\mathcal{P}}{dN} = -V_T'(H)C\tau\mathcal{P}\langle\kappa^2\rangle \quad (24)$$

so in the homogeneous first-order approximation $\frac{d\mathcal{P}}{dN} < 0$. This result is important to test the model assumptions in relation to the ac-dynamic roughening of the DW observed experimentally.

## VII. NUMERICAL VALIDATION OF THE MODEL

To analyze the DW dynamics, and also to validate the phenomenological model of the previous section, we numerically solve a standard time-

dependent field-driven two-dimensional scalar ferromagnetic Ginzburg-Landau model (TDGL) with disorder [5–8],

$$\eta \partial_t \phi = c \nabla^2 \phi + \epsilon_0 [(1 + r(x, y))\phi - \phi^3] + h_t, \quad (25)$$

where $\epsilon_0 > 0$, $\phi \equiv \phi(x, y, t)$ models the out-of-plane local magnetization, $h_t$ is a time-dependent driving field, and $r(x, y)$ an uncorrelated random-bond type of disorder of strength $r_0$. The disorder is specified by

$$\overline{r(x,y)} = 0,$$
$$\overline{r(x',y')r(x,y)} = r_0^2 \delta(x - x')\delta(y - y'), \quad (26)$$

where $\overline{...}$ denotes average over disorder realizations.

Starting the dynamics with a saturated magnetization $\phi \sim -\phi_s$ and then nucleating a compact domain with saturation magnetization $\phi_s \sim \phi_s$ a well defined closed DW with a width $\delta \sim \sqrt{c/\epsilon_0}$ and surface tension $\sigma \sim \sqrt{c\epsilon_0}$ is formed and driven by $h_t$ in a disordered environment. The DW position is described by an evolving closed curve $\Gamma_t$ described by the points $\mathbf{r}_s \in \Gamma_t$ such that $\phi(\mathbf{r}_s) = 0$. It can be shown that the heterogeneity of Eqs.(26) do not destroy the ferromagnetic state for small enough $r_0$ but induces a spatially uncorrelated and isotropic DW pinning with a correlation length of the order of the DW width $\delta$ [6]. On the other hand, in the absence of pinning and in presence of a uniform and constant field $h$ an initially flat DW moves steadily with a velocity $V_T(h) = mh$, where $m \approx \eta/\delta$ is the DW mobility.

This TDGL scalar model is an oversimplification of the micro-magnetic vector model dynamics. Nevertheless, it can capture the competition between elasticity and disorder in driven DWs which is at the root of many mesoscopic or macroscopic phenomena. It has the disadvantage of being computationally expensive compared to a direct simulation of elastic interface DW models, but it has the advantage that can be used for studying DWs with multi-valued DW displacement fields, and used to study plastic effects such as pinch-off loops. Here we will use it exclusively to test the analytical predictions of the previous section, and also to emulate the experimental protocol numerically. To Solve the TDGL we use a standard parallelized finite difference technique.

### A. Spontaneous and ac-assisted collapse dynamics without pinning

When $r_0 = 0$ and $h_t = 0$ we can verify that the curvature-driven area collapse occurs at a constant rate $dA_t/dt = -2\pi Cm \equiv \pi\sqrt{c\epsilon_0}/\phi_s$, regardless of the initial condition (only provided it is a compact domain with resonable small distortions compared to $\delta$). In Fig.5 we show the spontaneous time-evolution of three different initial conditions that we reminiscently label SARSCOV2, DOG and CIRCLE. The relative change of areas in each case is shown in Fig.6(a). The prediction $dA_t/dt = -\pi\sqrt{c\epsilon_0}/\phi_s$ is accurately satisfied for the three initial conditions, from the initial domain almost until it disappears. In contrast, the evolution of the perimeter *does* depend on the initial condition as can be appreciated in Fig.6(b). The lifetime of a domain is nevertheless only determined by its initial area. We note that the circular case is special because we can get an analytical expression for the perimeter evolution. This is so because $\mathcal{A} = \mathcal{P}^2/4\pi$ and then we have $\mathcal{A} = \mathcal{A}_0 - 2\pi Cmt$, and $\mathcal{P} = \sqrt{\mathcal{P}_0^2 - 8\pi^2 Cmt}$, a shape that is appreciated in Fig.6(b). The TDGL model hence captures well the geometric and dynamic features about the general elastic DW dynamics.

Let us now check the prediction for the AC-assisted collapse of Eq. (21), which can be written as,

$$-\frac{d}{dN}\left[\frac{\mathcal{A} + \frac{\tau}{4}V_T(H)\mathcal{P}}{2\pi V_T'(H)\tau}\right] = \frac{d\Lambda}{dN} \approx C. \quad (27)$$

with $C \approx \sigma/2\phi_s$. Note that this equation contains the $h_t = 0$ spontaneous collapse. In that case, the steady-state velocity evaluated at the AC-amplitude is $V_T(H = 0) = 0$ and $V_T'(0) = m$ (the mobility), so the area $\mathcal{A}$ decays at a constant rate. If the AC-field has a non-zero amplitude $H$ however, it is the quantity $\Lambda$ what decays at the same constant rate of the spontaneous area collapse, but not the area $\mathcal{A}$ alone.

To check Eq.(27) we apply, as in the experiment, a small square-pulse AC field of small amplitud $H$, with an AC period such that $V_T(H)\tau \equiv mH\tau \ll L_t$, with $L_t$ the linear size of the domain during its evolution. We use the same three initial conditions of Fig.5 but evolving them with the superimposed AC-field. In Fig.7 we show the evolution of the relative change of $\mathcal{A}_N$ and $\Lambda_N$ vs the number $N$ of AC-cycles for a $512 \times 512$ numerical grid. As it can be observed $\mathcal{A}$ does not decay at a constant rate but $\Lambda$ does, and with the same rate the area spontaneously decays. Note that for the circular case, in contrast with other initial conditions, we can compute $\mathcal{A}_N$ analytically:

$$\mathcal{A}_N = \mathcal{A}_0 - 2\pi CmN\tau + \frac{\tau}{4}mH\left[\sqrt{\mathcal{P}_0^2 - 8\pi^2 CmN\tau} - \mathcal{P}_0\right]. \quad (28)$$

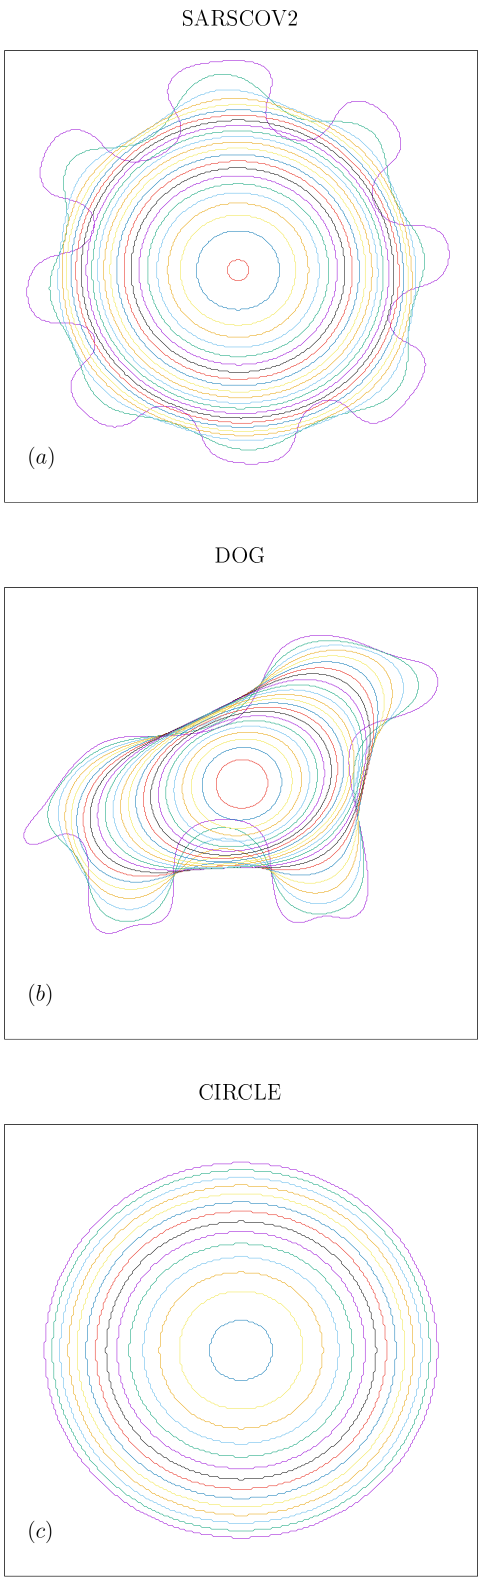


Figure 5. Three different initial conditions for the closed DW and its spontaneous collapse dynamics, driven by surface tension. In all cases, the domain area monotonically shrinks, transforming into a circle before disappearing.

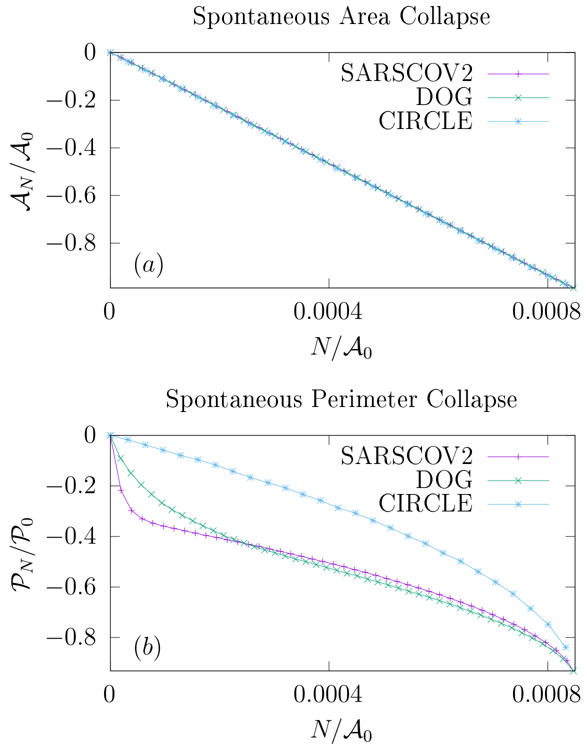


Figure 6. Area (a) and Perimeter (b) evolution for the spontaneous collapse of the initial domains of Fig.5, in the absence of pinning. The area decay-rate is independent of the initial conditions due to the linear local and instantaneous DW response $v \propto mC\kappa$ at each point of the DW with local curvature $\kappa$, and to the topological invariant $\int_{\Gamma_t} \kappa_t(s)ds = -2\pi$ of the DW Jordan curve $\Gamma_t$.

This clearly shows that under the AC assisted collapse it is $\Lambda$ and not $\mathcal{A}$ what linearly decrease with time and as can be appreciated in Fig.7(c) the agreement is excellent if there is no heterogeneity at the coarse grained TDGL scale, i.e. $r_0 = 0$. The formula Eq.(27) is actually accurately verified in the absence of pinning for arbitrary compact initial conditions, provided the AC field is such that a small relative changes $A_{N+1} - A_N \ll A_N$.

## B. AC-assisted collapse dynamics with pinning

Eq.(27) was derived neglecting heterogeneity at the coarse-grained scale. Note that this is not equivalent to completely neglect disorder, because it can be already present in the form of $V_T$. To study how this large scale heterogeneity affects the pre-

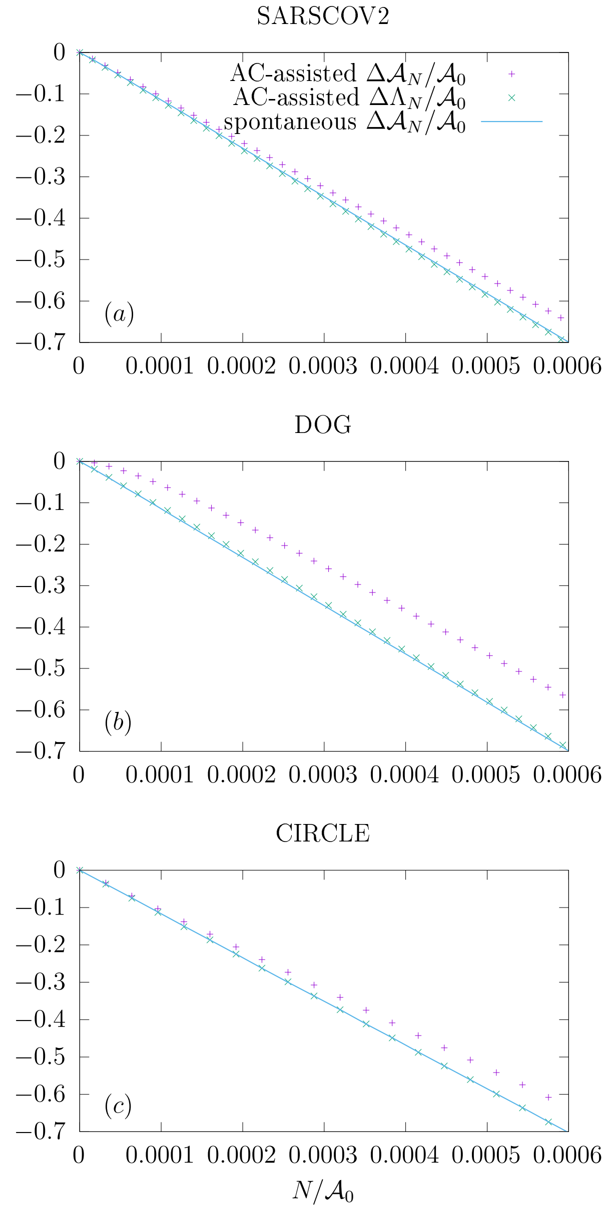


Figure 7. When the surface-tension collapse is assisted by an AC-field the rate of area decay $\Delta\mathcal{A}_N/\mathcal{A}_0$ is not constant as in the spontaneous collapse but depends on the initial condition. The combination $\Delta\Lambda \propto \Delta\mathcal{A} + V_T(h_0)(\tau/4)\Delta P$ however, where $\Delta\mathcal{P} = \mathcal{P}_N - \mathcal{P}_0$ is the perimeter change and $V_T(h_0)\tau/4$ is the DC domain wall displacement in 1/4 of an AC-period $\tau$ for a constant field $h_0$ is approximately constant if $A_{N+1} - A_N \ll A_N$. In the absence of pinning we have $V_T(h_0) = h_0/\eta w$. The three panels (a), (b) and (c) correspond to geometrical observables of the initial conditions of Fig.5. In all cases $\Delta\Lambda$ decreases with the same constant rate as in the spontaneous area collapse.

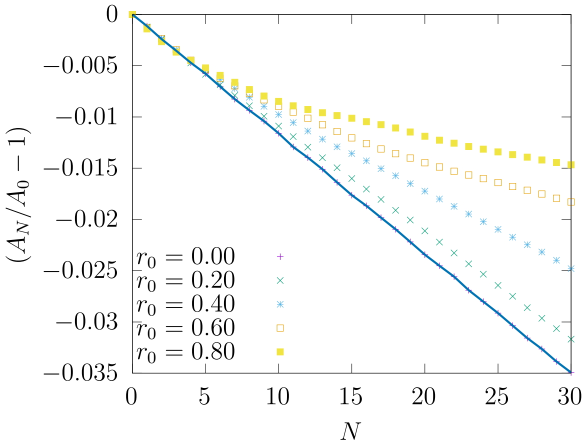


Figure 8. AC-assisted collapse of a circular domain area $A_N$ as a function of the number $N$ of AC-cycles for different disorder strengths $r_0$. The solid-line corresponds to the case without disorder.

diction of Eq.(27) we now monitor the AC-assisted area collapse for pinning of increasing strength $r_0$ in the TDGL equations (25) and (26).

In Fig.8 we show results of TDGL numerical simulations for an initial circle of radius $R = 400$ in a $1024 \times 1024$ computational grid for increasing $r_0$, including $r_0 = 0$ (no disorder) as a reference. As it can be appreciated, there is a deviation from the prediction of Eq.(27) (indicated with the solid line) increasing $N$. The deviation is upwards, i.e. slowing down the area collapse. Interestingly however, the initial decay for small $N$ is well defined and identical for all $r_0$. This initial slip here corresponds to the one of the $r_0 = 0$ case, and thus determined by the coarse-grained mobility which is simply the free-flow value $m \approx \eta/\delta$ in our simulations. Nevertheless, the prediction of Eq.(27) is expected to hold in non-linear regimes as well, provided the *coarse-grained* heterogeneity can be neglected.

The curves of Fig.8 for increasing $r_0$ are similar to the ones observed experimentally as a function of the decreasing AC fields, where $\tau$ is adjusted so to fix $V_T(H)\tau$. This makes sense as the faster the DW motion the less effective is the pinning and the large-scale dynamic roughening.

## VIII. HOW STABLE ARE CIRCULAR DOMAINS?

With our phenomenological model it is interesting to make rough estimates of the time needed for a circular domain of initial radius $R_0$ to collapse spontaneously, i.e. at $H = 0$, only acted by the Young-Laplace force at ambient temperature. Assuming a roughly circular domain we can directly integrate Eq.(5) in a circle of radius $R_t$ and use $A_t \approx \pi R_t^2$. Doing so we get the simple closed equation

$$\frac{dR_t}{dt} \approx V_T(H - C/R) = -V_T(C/R_t) \tag{29}$$

for the time dependent radius $R_t$, where $V_T(C/R_t)$ can be a linear or non-linear function depending on the magnitude of $C/R_t$, the strenght of the disorder and the temperature.

### A. Without pinning

It is interesting to consider first the non-disordered case, $v(H) \sim mH$, with $m$ the DW mobility. The equation then reduces to the Cahn-Allen equation, $\frac{dR_t}{dt} = -m\frac{C}{R_t}$. The solution for this case is $R_t^2 = R_0^2 - 2mCt$. Defining a "half-radius" lifetime $\tau_{1/2}$ such as $R_{\tau_{1/2}} = R_0/2$ we have $R_0^2/4 = R_0^2 - 2mC\tau_{1/2}$ and then

$$\tau_{1/2} = \frac{3R_0^2}{8mC} \tag{30}$$

Using the estimate for sample S1 $C = \sigma/2M_s \approx 0.001$ Oe cm and $m = 10$cm/s Oe, we obtain $\tau_{1/2}(R_0) = 37.5$ cm$^{-2}$ $R_0^2$. To get an idea, a $R_0 = 50\mu$m bubble has $\tau_{1/2} = 1$ ms. This means that in the absence of disorder the collapse of a millimetric bubble should be observable in a scale of seconds.

Rather strikingly, the result of Eq.(30) is valid for *any* initial simple closed curve $\Gamma(t)$ describing the DW at time $t$, not only for a circular one. The area indeed satisfies

$$\frac{dA}{dt} = \int_{\Gamma_t} v_n ds = Cm \int_{\Gamma_t} \kappa_t ds = -2\pi Cm, \tag{31}$$

where $\kappa_t$ is the instantanous signed local curvature, $v_n \equiv mC\kappa$ and in the last equality we have used the topological index of the curve Jordan-curve $-2\pi = \int_{\Gamma_t} \kappa_t \, ds$ (see for instance [9]). Therefore

$$A_t = A_0 - 2\pi Cmt \tag{32}$$

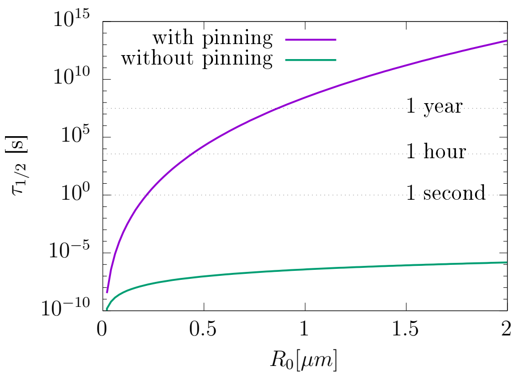


Figure 9. Lifetimes of circular magnetic domains in Pt/Co/Pt films in the absence of applied fields, for different initial radii $R_0$.

leading to equation 30 if we define $A(t) = \pi R_t^2$. Therefore, the lifetime *only* depends on the initial area but not the initial shape. Similarly, for the perimeter we can write the general equation

$$\frac{dP}{dt} = \int_{\Gamma(t)} v_n \kappa ds = Cm \int_{\Gamma(t)} \kappa^2 ds, \tag{33}$$

but we can not solve it without knowing the time dependent curvature $\kappa_t$. We can solve it for the circular case however, $\kappa_t = -1/R_t$, and its solution is equivalent to Eq.(32), using that $A_t = \pi R_t^2 = P_t^2/(4\pi)$. Eqs.(31) and (33) are well known results from the curve-shortening flow theory in differential geometry.

### B. With pinning

In the presence of disorder, we find that $C/R_0 \ll H_d$ for all PMOKE observable ($R_0 > 1\mu m$) bubbles. This means that the collapse dynamics occurs in the thermally activated creep regime. Using the circular approximation we again get a closed equation for $R_t$,

$$\frac{dR_t}{dt} = -V_T\left(\frac{C}{R_t}\right) \approx -v_0 e^{-\frac{T_d}{T}\left(\frac{R_t}{R_d}\right)^\mu} \tag{34}$$

where we have defined $R_d \equiv C/H_d$ and used that $C/R_d \gg C/R_t$ in order to use the creep law $V_T(H) = v_0 \exp[-(T_d/T)(H_d/H)^\mu]$ with $T_d$ and $H_d$ the characteristic temperature and depinning field respectively. Note that the creep condition is equivalent to $R_t \gg R_d$, in consistence with the crossover from the Larkin regime to the random-manifold regime of the DW. The resulting equation is highly

non-linear due to the creep response. For the "half-radius life" $\tau_{1/2}$ we obtain

$$\tau_{1/2}(R_0) \approx \int_{R_0/2}^{R_0} dr\; v_0^{-1} e^{\frac{T_d}{T}\left(\frac{r}{R_d}\right)^{\mu}}. \quad (35)$$

This integral can be done analytically. It is however clear that since we are interested in $R_0 \gg R_d$ and $T_d > T$ (for Pt/Co/Pt films we have for instance $R_d \approx 0.1\mu m$ and $T_d/T \approx 3.4$ for $T \sim 293K$ and using $T_d \sim 1000$K [10]), the integral will be dominated by the initial radius $r \sim R_0$,

$$\tau_{1/2}(R_0) \approx \frac{R_0}{V_T(C/R_0)} \quad (36)$$

Therefore, while the dependence with the initial radius is quadratic in the absence of disorder (Eq.(30)), with disorder it is a strechted-exponential. To get an estimate one can naively extrapolate the velocity field characteristics $V_T(H)$ to a very small field $H = C/R_0$. Doing so and using $C \approx 0.001$ Oe cm we obtain the result of Fig.9.

The above extrapolation must be done with care because finite-size effects will be very important precisely in the limit of very low applied fields where the creep-law takes a different form. The cut-off size of creep events grows as $L_{opt} \sim L_d(H_d/H)^{\nu}$ with the applied field $H$, and the associated barrier scale as $U_{opt} \sim L_{opt}^{\theta} \sim H^{-\theta\nu} = H^{-\mu}$. When $H$ is such that $L_{opt} > R_0$ we have finite-size effects [11] and the creep-law crossovers to normal Arrhenius activation over a size dependent barrier $R_0^{-\mu}$ correponding to a thermal nucleous of size $R_0$. For curvature driven creep finite size effects will be important when $L_{opt} \approx L_d(H_d R_0/C)^{\nu} = L_d(R_0/R_d)^{\nu} > R_0$ with $\nu = 3/4$. That is $(L_d/R_d)(R_0/R_d)^{\nu-1} > 1$. For Pt/Co/Pt films we have for instance $L_d/R_d \approx 4$ ($L_d \approx 0.04\mu m$ and $R_d \approx 0.01$), implying $(R_d/R_0) > 1$, which is not satisfied for observable bubbles where $R_0/R_d > 100$. This justifies the extrapolation used in Fig.9.

Domains in Pt/Co/Pt thin films with radii of the order or larger than on micrometer are already super-stable at ambient temperature. This means that it is difficult to observe a spontaneous curvature collapse using standard PMOKE microscopy at ambient temperature. Although the calculation was done for quasi-circular domains we expect a lifetime of the same order of magnitude for other domain shapes. Including the effect of dynamic roughening at large scales can make the dynamics even slower, as discussed in the previous section (see Fig.8) and in the experiment (see main text).


[1] C. P. Quinteros, S. Bustingorry, J. Curiale, and M. Granada, Appl. Phys. Lett. **112**, 262402 (2018).

[2] C. P. Quinteros, M. J. C. Burgos, L. J. Albornoz, J. E. Gómez, P. Granell, F. Golmar, M. L. Ibarra, S. Bustingorry, J. Curiale, and M. Granada, Journal of Physics D: Applied Physics **54**, 015002 (2020).

[3] J.-C. Rojas-Sánchez, P. Laczkowski, J. Sampaio, S. Collin, K. Bouzehouane, N. Reyren, H. Jaffrès, A. Mougin, and J.-M. George, Appl. Phys. Lett. **108**, 082406 (2016).

[4] P. J. Metaxas, J. P. Jamet, A. Mougin, M. Cormier, J. Ferré, V. Baltz, B. Rodmacq, B. Dieny, and R. L. Stamps, Phys. Rev. Lett. **99**, 217208 (2007).

[5] N. B. Caballero, E. E. Ferrero, A. B. Kolton, J. Curiale, V. Jeudy, and S. Bustingorry, Phys. Rev. E **97**, 062122 (2018).

[6] N. Caballero, E. Agoritsas, V. Lecomte, and T. Giamarchi, Phys. Rev. B **102**, 104204 (2020).

[7] P. C. Guruciaga, N. B. Caballero, V. Jeudy, J. Curiale, and S. Bustingorry, "Ginzburg-landau micromagnetic model to study domain wall dynamics in thin ferromagnetic systems," (2019), arXiv:1912.09392 [cond-mat.dis-nn].

[8] N. Caballero, "Degradation of domains with sequential field application," (2020), arXiv:2009.14205 [cond-mat.dis-nn].

[9] B. White, "Evolution of curves and surfaces by mean curvature," (2002), arXiv:math/0212407 [math.DG].

[10] J. Gorchon, S. Bustingorry, J. Ferré, V. Jeudy, A. B. Kolton, and T. Giamarchi, Physical Review Letters **113**, 027205 (2014).

[11] J.-C. Lee, K.-J. Kim, J. Ryu, K.-W. Moon, S.-J. Yun, G.-H. Gim, K.-S. Lee, K.-H. Shin, H.-W. Lee, and S.-B. Choe, Phys. Rev. Lett. **107**, 067201 (2011).
